# Supplementary material for: Emergence of the strong tunable linear Rashba spin-orbit coupling of two-dimensional hole gases in semiconductor quantum
Source: arXiv:2008.12523 source file (2020-09-19)
Supplement: Supplementary file 1 [file supplemental.pdf]

# Supplementary Information to: "Emergence of the strong tunable linear Rashba spin-orbit coupling of two-dimensional hole gases in semiconductor quantum wells"

Jia-Xin Xiong,[1,2] Shan Guan,[1,*] Jun-Wei Luo,[1,2,3,†] and Shu-Shen Li[1,2]

[1]*State Key Laboratory of Superlattices and Microstructures, Institute of Semiconductors,Chinese Academy of Sciences, Beijing 100083, China*

[2]*Center of Materials Science and Optoelectronics Engineering, University of Chinese Academy of Sciences, Beijing 100049, China*

[3]*Beijing Academy of Quantum Information Sciences, Beijing 100193, China*

* shan_guan@semi.ac.cn

† jwluo@semi.ac.cn

**Supplementary Note 1: Traditional 2D Hamiltonian by the k·p method.** According to bulk symmetry, the Hamiltonian to describe HH and LH states is[1]

$$H_{SO} = \beta_1 \mathbf{k} \times \mathbf{E} \cdot \mathbf{J} + \beta_2 \mathbf{k} \times \mathbf{E} \cdot \mathcal{J}, \tag{1}$$

where $\mathbf{J} = (J_x, J_y, J_z)$ and $\mathcal{J} = (J_x^3, J_y^3, J_z^3)$, with $J_x$, $J_y$, $J_z$ are the angular momentum matrices for $j = 3/2$. For QWs confined in the z-direction, where the external electric field is applied, Eq. 1 can be written as

$$H_{SO} = \beta_1 E_z \begin{bmatrix} 0 & 0 & i\frac{\sqrt{3}}{2}k_- & 0 \\ 0 & 0 & 0 & -i\frac{\sqrt{3}}{2}k_+ \\ -i\frac{\sqrt{3}}{2}k_+ & 0 & 0 & ik_- \\ 0 & i\frac{\sqrt{3}}{2}k_- & -ik_+ & 0 \end{bmatrix} + \beta_2 E_z \begin{bmatrix} 0 & -i\frac{3}{4}k_+ & i\frac{7\sqrt{3}}{8}k_- & 0 \\ i\frac{3}{4}k_- & 0 & 0 & -i\frac{7\sqrt{3}}{8}k_+ \\ -i\frac{7\sqrt{3}}{8}k_+ & 0 & 0 & i\frac{5}{2}k_- \\ 0 & i\frac{7\sqrt{3}}{8}k_- & -i\frac{5}{2}k_+ & 0 \end{bmatrix}, \tag{2}$$

with $k_\pm = k_x \pm ik_y$ in the basis $\{|\frac{3}{2}, +\frac{3}{2}\rangle, |\frac{3}{2}, -\frac{3}{2}\rangle, |\frac{3}{2}, +\frac{1}{2}\rangle, |\frac{3}{2}, -\frac{1}{2}\rangle\}$ as the HH and LH eigenstates. We can simply use the quasi-degenerate perturbation theory to judge the k splitting relationship, by reducing the $4 \times 4$ matrix to a $2 \times 2$ one. For the first term, the reduced Hamiltonian matrix element $\widetilde{H_{12}}$ keeps zero till the second-order perturbation, and appears to be non-zero at third-order perturbation ($\widetilde{H_{12}} = H'_{13}H'_{34}H'_{42} \propto k_-^3$). Hence the first term gives a cubic splitting $\Delta\varepsilon_{HH} \propto \beta_1 E_z k_\parallel^3$. For the second term, due to the appearance of non-zero matrix elements $H_{12} = -i\frac{3}{4}k_+$ and $H_{21} = i\frac{3}{4}k_-$, the splitting shows a linear relationship $\Delta\varepsilon_{HH} \propto \beta_2 E_z k_\parallel$. However, the prefactor $\beta_2$, originating from the isotropic $k \cdot p$ coupling between $\Gamma_8^v$ and $\Gamma_6^c$, is much smaller than the prefactor $\beta_1$, originating from the anisotropic $k \cdot p$ coupling between $\Gamma_8^v$ and remote conduction bands $\Gamma_7^c$ and $\Gamma_8^c$[1]. Consequently, the second term could be neglected, even for QWs grown in low-symmetric directions, and the Rashba spin splitting for HH exhibits a **k**-cubic relationship.

However, Eq. 1 is constructed under the bulk symmetry and the reduction from Eq. 1 to Eq. 2 results in a fictitiously higher symmetry for QWs, leading to the ignorance of mixings between pure bulk HH and LH states. In other words, the HH (LH) eigenstates are not pure bulk HH (LH) states, but so-called HH-type (LH-type) states with the bulk HH (LH) states dominating over tiny bulk LH (HH) states (Eq. 6). Notably, the second valence bands in QWs can also be of HH-type (see Figure 1 in the main text), determined by the strength of the space confinement effect (SCE). We next illustrate that the mixings between pure bulk HH and LH states lead to the mixing between the ground states (HH1) and the excited

states (HH2), finally resulting in the **k**-linear spin splitting.

**Supplementary Note 2: Effective 2D Hamiltonian in growth direction [001] QWs.** The Luttinger-Kohn Hamiltonian is commonly used to describe the valence bands. For z along [001] direction, it is given by[2]

$$\begin{aligned} H_{LK}^{[001]} =& \frac{\hbar^2}{2m_0}[(\gamma_1 + \frac{5\gamma_2}{2})k^2 - 2\gamma_2(k_x^2 J_x^2 + k_y^2 J_y^2 + k_z^2 J_z^2) \\ & - 4\gamma_3(\{k_x, k_y\}\{J_x, J_y\} + \{k_y, k_z\}\{J_y, J_z\} + \{k_z, k_x\}\{J_z, J_x\})]. \end{aligned} \tag{3}$$

Here the x and y directions are along with the crystallographic [100] and [010] directions, respectively. And $\gamma_1$, $\gamma_2$ and $\gamma_3$ are the Luttinger parameters with the values shown in Table I [3]. Next, we express the $H_{LK}^{[001]}$ in the basis $\{|+\frac{3}{2}\rangle, |-\frac{3}{2}\rangle, |+\frac{1}{2}\rangle, |-\frac{1}{2}\rangle\}$ as

$$H_{eff}^{[001]}(k_\pm, k_z) = \begin{bmatrix} \mu(\frac{\gamma_1+\gamma_2}{2}k_\parallel^2 + \frac{\gamma_1-2\gamma_2}{2}k_z^2) & 0 & -\sqrt{3}\mu\gamma_3 k_- k_z & -\frac{\sqrt{3}\mu}{2}(\eta k_-^2 + \delta k_+^2) \\ 0 & \mu(\frac{\gamma_1+\gamma_2}{2}k_\parallel^2 + \frac{\gamma_1-2\gamma_2}{2}k_z^2) & -\frac{\sqrt{3}\mu}{2}(\eta k_+^2 + \delta k_-^2) & \sqrt{3}\mu\gamma_3 k_+ k_z \\ -\sqrt{3}\mu\gamma_3 k_+ k_z & -\frac{\sqrt{3}\mu}{2}(\eta k_-^2 + \delta k_+^2) & \mu(\frac{\gamma_1-\gamma_2}{2}k_\parallel^2 + \frac{\gamma_1+2\gamma_2}{2}k_z^2) & 0 \\ -\frac{\sqrt{3}\mu}{2}(\eta k_+^2 + \delta k_-^2) & \sqrt{3}\mu\gamma_3 k_- k_z & 0 & \mu(\frac{\gamma_1-\gamma_2}{2}k_\parallel^2 + \frac{\gamma_1+2\gamma_2}{2}k_z^2) \end{bmatrix}, \tag{4}$$

where $\mu = \frac{\hbar^2}{m_0}$, $\eta = \frac{\gamma_2+\gamma_3}{2}$, $\delta = \frac{\gamma_2-\gamma_3}{2}$, $k_\pm = k_x \pm ik_y$, and $k_\parallel = \sqrt{k_x^2 + k_y^2}$. Considering the confinement$(-L/2 < z < L/2)$ as a hard wall, we can describe the envelope function using

$$\phi_n(z) = \sqrt{\frac{2}{L}} sin[\frac{n\pi(z + L/2)}{L}]. \tag{5}$$

In the presence of HH-LH mixing, the four basis states read

$$\begin{aligned} |\mathrm{HH1}_\pm\rangle &= a_1\phi_1(z)|\frac{3}{2}, \pm\frac{3}{2}\rangle + b_1\phi_1(z)|\frac{3}{2}, \mp\frac{1}{2}\rangle, \\ |\mathrm{HH2}_\pm\rangle &= a_2\phi_2(z)|\frac{3}{2}, \pm\frac{3}{2}\rangle + b_2\phi_2(z)|\frac{3}{2}, \mp\frac{1}{2}\rangle. \end{aligned} \tag{6}$$

Here, $|\mathrm{HH1}_\pm\rangle$ and $|\mathrm{HH2}_\pm\rangle$ denote the ground states (HH1) and the first excited states (HH2), respectively, with the subscripts "+" and "-" representing two different spin blocks of the contained spin states $|3/2, \pm 3/2\rangle$ at $\bar{\Gamma}$ point. Then, we obtain the effective 2D Hamiltonian in the presence of perpendicular external electric field written as

$$H_{eff}^{[001]} = \begin{bmatrix} \frac{\hbar^2 k_x^2}{2m_{1x}} + \frac{\hbar^2 k_y^2}{2m_{1y}} & 0 & eU_0E_z & -i\gamma_3C_0k_- \\ 0 & \frac{\hbar^2 k_x^2}{2m_{1x}} + \frac{\hbar^2 k_y^2}{2m_{1y}} & i\gamma_3C_0k_+ & eU_0E_z \\ eU_0E_z & -i\gamma_3C_0k_- & \frac{\hbar^2 k_x^2}{2m_{2x}} + \frac{\hbar^2 k_y^2}{2m_{2y}} + \Delta_0 & 0 \\ i\gamma_3C_0k_+ & eU_0E_z & 0 & \frac{\hbar^2 k_x^2}{2m_{2x}} + \frac{\hbar^2 k_y^2}{2m_{2y}} + \Delta_0 \end{bmatrix}, \tag{7}$$

where $U_0 = (a_g a_e + b_g b_e)\frac{16L}{9\pi^2}$ denotes the direct coupling strength to the external electric field, $C_0 = (a_g b_e - a_e b_g)\frac{8\sqrt{3}\mu}{3L}$ characterizes the mixing strength between the HH-type ground states and the HH-type excited states, and $\Delta_0$ is the energy separation between HH1 and HH2 states.

Next, we use the quasi-degenerate perturbation theory to reduce this $4 \times 4$ effective Hamiltonian and obtain the **k**-linear direct Rashba parameter. Analogous to the derivation in Ref.[4], the reduction of this Hamiltonian involves three steps. First, we split it into two parts, including the leading-order part and the perturbation part. Then we find a unitary matrix to diagonalize the leading-order Hamiltonian and obtain the transformed perturbation Hamiltonian. Finally, we use the standard quasi-degenerate perturbation theory to obtain the reduced effective Hamiltonian.

Table I. Luttinger parameters for several semiconductors[3].

| | GaAs | InAs | InSb | Si | Ge |
|---|---|---|---|---|---|
| $\gamma_1$ | 6.85 | 20.40 | 37.10 | 4.28 | 13.38 |
| $\gamma_2$ | 2.10 | 8.30 | 16.50 | 0.34 | 4.24 |
| $\gamma_3$ | 2.90 | 9.10 | 17.70 | 1.45 | 5.69 |

In the first step, considering the wavevector near the Brillion zone center, we split the $4 \times 4$ effective Hamiltonian $H_{4\times 4}^{eff}$ (Eq. 7) into the leading-order Hamiltonian

$$H_{4\times 4}^{0} = \begin{bmatrix} 0 & 0 & eU_0E_z & 0 \\ 0 & 0 & 0 & eU_0E_z \\ eU_0E_z & 0 & \Delta_0 & 0 \\ 0 & eU_0E_z & 0 & \Delta_0 \end{bmatrix}, \tag{8}$$

and the perturbation Hamiltonian

$$H_{4\times 4}^{'} = \begin{bmatrix} \frac{\hbar^2 k_x^2}{2m_{1x}} + \frac{\hbar^2 k_y^2}{2m_{1y}} & 0 & 0 & -i\gamma_3 C_0 k_- \\ 0 & \frac{\hbar^2 k_x^2}{2m_{1x}} + \frac{\hbar^2 k_y^2}{2m_{1y}} & i\gamma_3 C_0 k_+ & 0 \\ 0 & -i\gamma_3 C_0 k_- & \frac{\hbar^2 k_x^2}{2m_{2x}} + \frac{\hbar^2 k_y^2}{2m_{2y}} & 0 \\ i\gamma_3 C_0 k_+ & 0 & 0 & \frac{\hbar^2 k_x^2}{2m_{2x}} + \frac{\hbar^2 k_y^2}{2m_{2y}} \end{bmatrix}. \tag{9}$$

All the elements in the leading-order Hamiltonian $H_{4\times 4}^{0}$ are $eU_0E_z$ or $\Delta_0$, and all **k**-linear and **k**-squared terms are involved in the perturbation Hamiltonian $H_{4\times 4}^{'}$.

In the second step, we use the unitary matrix $\tilde{U}$ to perform the unitary transformation $\tilde{U}^{\dagger}H_{4\times4}^{eff}\tilde{U}$. The unitary matrix can be written as

$$\tilde{U}=\begin{bmatrix} cos\theta & 0 & sin\theta & 0 \\ 0 & -cos\theta & 0 & sin\theta \\ -sin\theta & 0 & cos\theta & 0 \\ 0 & sin\theta & 0 & cos\theta \end{bmatrix}, \tag{10}$$

where

$$\begin{aligned} cos\theta &= \frac{\Delta_0+\Delta^{'}}{\sqrt{(\Delta_0+\Delta^{'})^2+(2eU_0E_z)^2}}, \\ sin\theta &= \frac{2eU_0E_z}{\sqrt{(\Delta_0+\Delta^{'})^2+(2eU_0E_z)^2}}, \end{aligned} \tag{11}$$

with

$$\Delta^{'}=\sqrt{\Delta_0^2+(2eU_0E_z)^2}. \tag{12}$$

Then we obtain the transformed leading-order Hamiltonian [omitting the constant energy shift $(\Delta_0-\Delta^{'})/2$]

$$\tilde{H}_{4\times4}^{(0)}=\tilde{U}^{\dagger}H_{4\times4}^{0}\tilde{U}=\begin{bmatrix} 0 & 0 & 0 & 0 \\ 0 & 0 & 0 & 0 \\ 0 & 0 & \Delta^{'} & 0 \\ 0 & 0 & 0 & \Delta^{'} \end{bmatrix}, \tag{13}$$

and the transformed perturbation Hamiltonian

$$\tilde{H}_{4\times4}^{'}=\tilde{U}^{\dagger}H_{4\times4}^{'}\tilde{U}=\begin{bmatrix} E_1 & -i\gamma_3C_0k_-sin2\theta & T & -i\gamma_3C_0k_-cos2\theta \\ i\gamma_3C_0k_+sin2\theta & E_1 & i\gamma_3C_0k_+cos2\theta & -T \\ T & -i\gamma_3C_0k_-cos2\theta & E_2 & -i\gamma_3C_0k_-sin2\theta \\ i\gamma_3C_0k_+cos2\theta & -T & i\gamma_3C_0k_+sin2\theta & E_2 \end{bmatrix}, \tag{14}$$

where

$$\begin{aligned} E_1 =&(\frac{\hbar^2k_x^2}{2m_{1x}}+\frac{\hbar^2k_y^2}{2m_{1y}})cos^2\theta+(\frac{\hbar^2k_x^2}{2m_{2x}}+\frac{\hbar^2k_y^2}{2m_{2y}})sin^2\theta, \\ E_2 =&(\frac{\hbar^2k_x^2}{2m_{1x}}+\frac{\hbar^2k_y^2}{2m_{1y}})sin^2\theta+(\frac{\hbar^2k_x^2}{2m_{2x}}+\frac{\hbar^2k_y^2}{2m_{2y}})cos^2\theta, \\ T =&[(\frac{\hbar^2k_x^2}{4m_{1x}}+\frac{\hbar^2k_y^2}{4m_{1y}})-(\frac{\hbar^2k_x^2}{4m_{2x}}+\frac{\hbar^2k_y^2}{4m_{2y}})]sin2\theta. \end{aligned} \tag{15}$$

In the third step, we use the standard second-order quasi-degenerate theory to obtain the reduced $2 \times 2$ effective Hamiltonian

$$
\begin{aligned}
H_{2\times 2}^{eff} =& [(\frac{\hbar^2 k_x^2}{4m_{1x}} + \frac{\hbar^2 k_y^2}{4m_{1y}}) + (\frac{\hbar^2 k_x^2}{4m_{2x}} + \frac{\hbar^2 k_y^2}{4m_{2y}})] + \frac{\Delta_0}{\Delta'}[(\frac{\hbar^2 k_x^2}{4m_{1x}} + \frac{\hbar^2 k_y^2}{4m_{1y}}) - (\frac{\hbar^2 k_x^2}{4m_{2x}} + \frac{\hbar^2 k_y^2}{4m_{2y}})] \\
& - \frac{\Delta_0^2 \gamma_3^2 C_0^2 (k_x^2 + k_y^2)}{(\Delta')^3} + \frac{2e\gamma_3 C_0 U_0 E_z}{\Delta'}(k_x \sigma_y - k_y \sigma_x).
\end{aligned} \tag{16}
$$

We illustrate that only the third term in Eq. 16 is the first-order result, and the other two terms are the second-order results. Obviously, for the **k**-linear terms, the first-order perturbation provides sufficiently reliable **k**-linear results. Consequently, the direct Rashba parameter has the form

$$
\alpha_R = \frac{2e\gamma_3 C_0 U_0 E_z}{\sqrt{\Delta_0^2 + 4e^2 U_0^2 E_z^2}}, \tag{17}
$$

given by the first-order coupling to the external electric field. If the eigenstates were pure HH states ($b_1 = b_2 = 0$), we would obtain $C_0 = 0$ and $U_0 = 0$, and thus $\alpha_R = 0$. If $m_{1x} = m_{2x}$ and $m_{1y} = m_{2y}$ and one ignores the second-order terms, the effective Hamiltonian can be written as

$$
H_{2\times 2}^{[001]} = (\frac{\hbar^2 k_x^2}{2m_{1x}} + \frac{\hbar^2 k_y^2}{2m_{1y}}) + \alpha_R^{[001]}(k_x \sigma_y - k_y \sigma_x). \tag{18}
$$

**Supplementary Note 3: Effective 2D Hamiltonian in growth direction [110] QWs.** For [110] direction, the Luttinger-Kohn Hamiltonian reads[2]

$$
\begin{aligned}
H_{LK}^{[110]} =& \frac{\hbar^2}{2m_0}[(\gamma_1 + \frac{5\gamma_2}{2})k^2 - \gamma_2(2k_x^2 J_x^2 + k_y^2 J_y^2 + k_z^2 J_z^2) - \gamma_2(k_y^2 J_z^2 + k_z^2 J_y^2 + 4\{k_y, k_z\}\{J_y, J_z\}) \\
& - 4\gamma_3(\{k_x, k_y\}\{J_x, J_y\} + \{k_z, k_x\}\{J_z, J_x\}) - \gamma_3(k_y^2 - k_z^2)(J_y^2 - J_z^2)].
\end{aligned} \tag{19}
$$

Here the x and y directions are along with the crystallographic [001] and [1$\bar{1}$0] directions, respectively. In the basis $\{|\frac{3}{2}, +\frac{3}{2}\rangle, |\frac{3}{2}, -\frac{3}{2}\rangle, |\frac{3}{2}, +\frac{1}{2}\rangle, |\frac{3}{2}, -\frac{1}{2}\rangle\}$, the $H_{LK}^{[110]}(k_\pm, k_z)$ is written as

$$
H_{eff}^{[110]}(\mathbf{k}) = \frac{\mu}{\mathbf{2}} \begin{bmatrix} M_1 & 0 & 2\sqrt{3}k_z(-\gamma_3 k_x + i\gamma_2 k_y) & T_1 + \sqrt{3}\delta k_z^2 \\ 0 & M_1 & T_1^\dagger + \sqrt{3}\delta k_z^2 & 2\sqrt{3}k_z(\gamma_3 k_x + i\gamma_2 k_y) \\ 2\sqrt{3}k_z(-\gamma_3 k_x - i\gamma_2 k_y) & T_1 + \sqrt{3}\delta k_z^2 & M_2 & 0 \\ T_1^\dagger + \sqrt{3}\delta k_z^2 & 2\sqrt{3}k_z(\gamma_3 k_x - i\gamma_2 k_y) & 0 & M_2 \end{bmatrix}. \tag{20}
$$

with $T_1 = \gamma_2\left(\frac{\sqrt{3}k_y^2}{2} - \sqrt{3}k_x^2\right) + 2i\sqrt{3}\gamma_3 k_x k_y + \frac{1}{2}\sqrt{3}\gamma_3 k_y^2$, $M_1 = -\frac{3}{2}(\gamma_2 k_x^2 + (2\gamma_2 - \gamma_3)k_y^2 + (2\gamma_2 + \gamma_3)k_z^2)$ and $M_2 = -\frac{7}{2}\gamma_2 k_x^2 - (2\gamma_2 + \frac{3}{2}\gamma_3)k_y^2 + (\frac{3}{2}\gamma_3 - 2\gamma_2)k_z^2$. By assuming $k_x = k_y = 0$, one can see that there is an intrinsic mixing of HH and LH, which is proportional to $\delta \times k_z^2$.

Similarly, we construct the basis states in the presence of HH-LH mixing as that of [001]-oriented QW in Eq. 6 and obtain the effective 2D Hamiltonian under the perpendicular external electric field for [110]-oriented QWs

$$H_{eff}^{[110]} = \begin{bmatrix} \frac{\gamma_3^2\hbar^2k_x^2}{2m_{1x}} + \frac{\gamma_2^2\hbar^2k_y^2}{2m_{1y}} & 0 & eU_0E_z & -iC_0(\gamma_3k_x - i\gamma_2k_y) \\ 0 & \frac{\gamma_3^2\hbar^2k_x^2}{2m_{1x}} + \frac{\gamma_2^2\hbar^2k_y^2}{2m_{1y}} & iC_0(\gamma_3k_x + i\gamma_2k_y) & eU_0E_z \\ eU_0E_z & -iC_0(\gamma_3k_x - i\gamma_2k_y) & \frac{\gamma_3^2\hbar^2k_x^2}{2m_{2x}} + \frac{\gamma_2^2\hbar^2k_y^2}{2m_{2y}} + \Delta_0 & 0 \\ iC_0(\gamma_3k_x + i\gamma_2k_y) & eU_0E_z & 0 & \frac{\gamma_3^2\hbar^2k_x^2}{2m_{2x}} + \frac{\gamma_2^2\hbar^2k_y^2}{2m_{2y}} + \Delta_0 \end{bmatrix}. \tag{21}$$

Finally, using the quasi-degenerate perturbation theory (similar to the derivation of [001]-oriented QWs), we obtain the **k**-linear direct Rashba splitting term, which takes the form of $\alpha_R^{[110]} = \frac{2e\gamma_3C_0U_0E_z}{\sqrt{\Delta_0{}^2+4e^2U_0{}^2E_z^2}}$ for $k_x$ and $\alpha_R^{[110]} = \frac{2e\gamma_2C_0U_0E_z}{\sqrt{\Delta_0{}^2+4e^2U_0{}^2E_z^2}}$ for $k_y$.

It is worth noting that the LH1 subband states can also contribute to the **k**-linear Rashba spin splitting. Taking LH1 subbands into account, we expand the number of basis states from four to six as $\{|\mathrm{HH1}_+\rangle, |\mathrm{HH1}_-\rangle, |\mathrm{HH2}_+\rangle, |\mathrm{HH2}_-\rangle, |\mathrm{LH1}_+\rangle, |\mathrm{LH1}_-\rangle\}$, where $|LH1_\pm\rangle = a_3\phi_1(z)|\frac{3}{2}, \pm\frac{3}{2}\rangle + b_3\phi_1(z)|\frac{3}{2}, \mp\frac{1}{2}\rangle$ represent the LH1 subband states. Following the standard approach, we obtain an additional **k**-linear Rashba parameter $\alpha_{R,con}^{[110]} \propto \frac{e\gamma_3E_z}{\Delta E_{g,e}\times\Delta E_{g,e_1}}$ for $k_x$, where $\Delta E$ denotes the energy separation between the corresponding two subband states at $\bar{\Gamma}$ point in the presence of the electric field. This additional **k**-linear Rashba splitting comes from a third-order effect and hence is smaller than our discovered direct Rashba splitting.

**Supplementary Note 4: Calculated results of [110]-oriented GaAs/AlAs QWs.** The **k**-linear Rashba SOC also exists in GaAs/AlAs QWs. As shown in Figure 1, the Rashba spin splitting of [110]-oriented $GaAs_{20}/AlAs_{20}$ QWs exhibits a **k**-linear relationship as well, where the Rashba parameter reaches the value of 31 $meV\mathring{A}$. Figure 2 shows the relationship between **k**-linear Rashba parameters and quantum well thickness and electric field, comparing the parameters of [110]-oriented GaAs/AlAs QWs and [110]-oriented Ge/Si QWs. We find that the Rashba parameters of GaAs/AlAs QWs are almost twice as large as Ge/Se QWs, but their energy separations are close to each other (Figure 3). Using our proposed model, we mainly attribute to the different material-dependent LK parameter $\gamma_3$,

where $\gamma_3$(Ge)=5.69 is about twice as large as $\gamma_3$(GaAs)=2.90[5]. The results of GaAs/AlAs QWs further improve the reliability of our model.

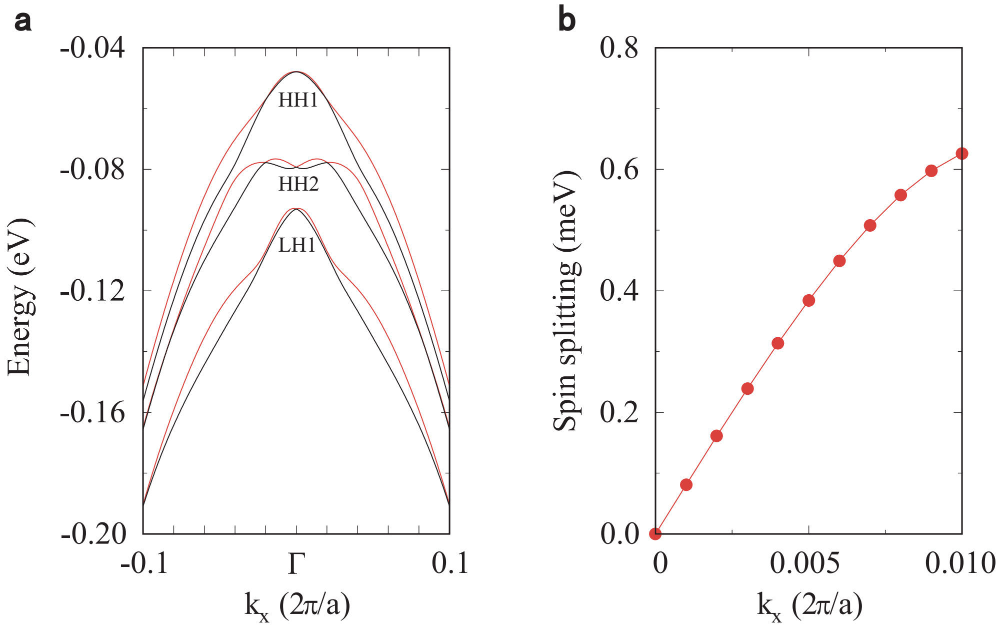


Figure 1. **a** Calculated energy dispersion of valence subbands and **b** spin splitting of HH1 for [110]-oriented $(GaAs)_{20}/(AlAs)_{20}$ QWs. The external perpendicular electric field is $E_z$=100 kV/cm. The x-direction is along the crystalline [001] direction. The labels HH1, HH2, LH1 in **a** represent the main components of each Kramers pair of valence subband states at Γ point, respectively.

## References

[1] Winkler, R. Rashba spin splitting in two-dimensional electron and hole systems. Phys. Rev. B **62**, 4245 (2000).

[2] Kloeffel, C., Rančić, M. J. & Loss, D. Direct Rashba spin-orbit interaction in Si and Ge nanowires with different growth directions. Phys. Rev. B **97**, 235422 (2018).

[3] Marcellina, E., Hamilton, A. R., Winkler, R. & Culcer, D. Spin-orbit interactions in inversion-asymmetric two-dimensional hole systems: A variational analysis. Phys. Rev. B **95**, 075305 (2017).

[4] Kloeffel, C., Trif, M. & Loss, D. Strong spin-orbit interaction and helical hole states in Ge/Si nanowires. Phys. Rev. B **84**, 195314 (2011).

[5] Winkler, R. Spin-Orbit Coupling Effect in Two-Dimensional Electron and Hole Systems. (Springer, 2003).

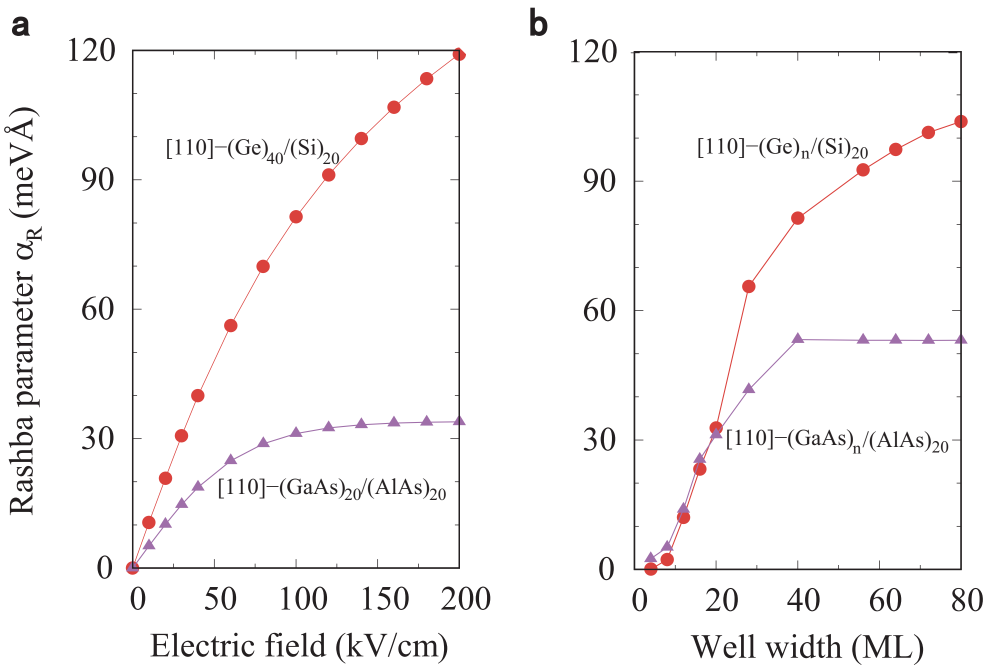


Figure 2. Calculated **k**-linear hole Rashba parameters $\alpha_R$ along the $k_x$ direction in [110]-oriented GaAs/AlAs QWs and [110]-oriented Ge/Si QWs as a function of **a** electric field strength with fixed well thickness, and **b** well thickness under an electric field of 100 kV/cm, respectively. (For GaAs/AlAs QWs, the number of the subscript denotes the number of bilayers.) Note that a larger electric field strength than 200 kV/cm is not experimentally available, hence the results are not shown.

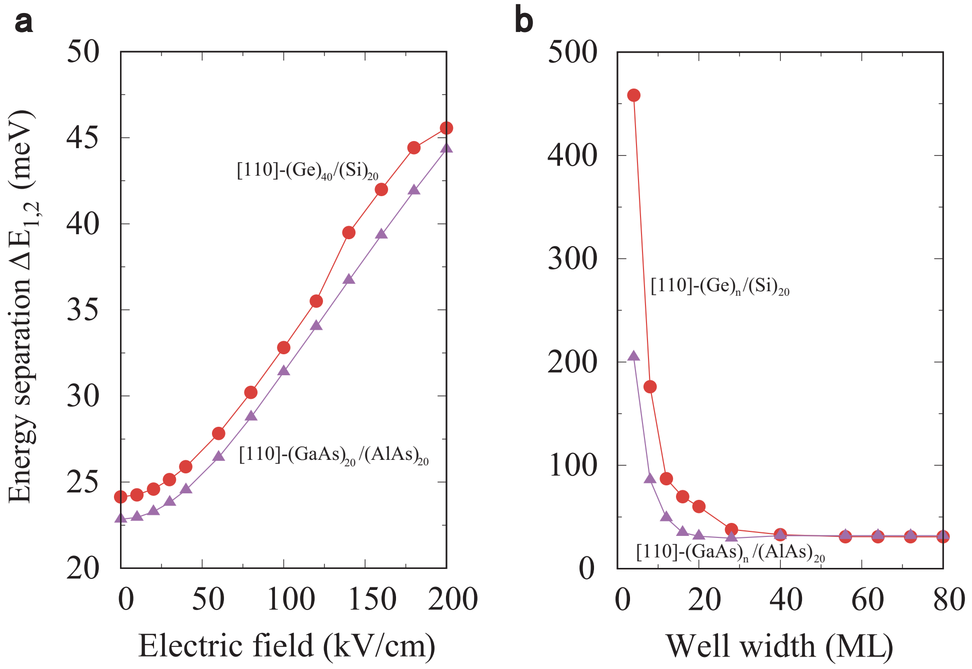


Figure 3. Energy separation $\Delta E_{1,2} = \sqrt{\Delta_0^2 + 4e^2 U_0^2 E_z^2}$ between HH1 and HH2 states at Γ point in [110]-oriented GaAs/AlAs QWs and [110]-oriented Ge/Si QWs as a function of **a** electric field strength, and of **b** well thickness with applied 100 kV/cm electric field, respectively.
